# Supplementary material for: Sparse-Tuning: Adapting Vision Transformers with Efficient Fine-tuning and Inference
Source: arXiv:2405.14700 source file (2025-12-18)
Supplement: Supplementary file 1 [file 6_appendix.tex]

\clearpage
\setcounter{page}{1}
\maketitlesupplementary

In the appendix, we provide detailed implementation information. We also present additional experiments to further analyze our Sparse-Tuning. We 
present PyTorch-like pseudocode to facilitate easy reproduction and extension by researchers. Finally, we include additional visualizations of Token Compression (TC) achieved through Sparse-Tuning.

\section{Implementation Details}
\label{sup:imple}

\noindent \textbf{Experimental settings on VTAB-1K.}
Following previous works \cite{jiang2024res-tuning,jia2022vpt}, we fine-tune the model for 100 epochs on each dataset in VTAB-1K~\cite{zhai2019vtab}. We \emph{do not} use any data augmentation strategy in these experiments. We adopt the AdamW \cite{loshchilov2017decoupled} optimizer. The base learning rate is set to 0.01 and gradually decays to 0 based on a cosine schedule \cite{loshchilov2016sgdr}.

\noindent \textbf{Experimental settings on complete image datasets.}
We use the settings in Table~\ref{tab:exp_image_complete} to fine-tune the ViT with the proposed Sparse-Tuning. Experiments on other parameter-efficient methods such as AdaptFormer \cite{chen2022adaptformer}, LoRA \cite{hu2021lora}, and VPT \cite{jia2022vpt} also follow the settings \cite{zhao2024dyt} in Table~\ref{tab:exp_image_complete}.

\begin{table}[ht]
\caption{Experimental settings for complete image datasets. We present the hyperparameters in Sparse-Tuning.}\label{tab:settings}
\label{tab:exp_image_complete}
\addtolength{\tabcolsep}{12pt}

    \centering
    \scriptsize
    
    \vspace{2mm}
\begin{tabular}{l  c}
\toprule
Configuration & {CIFAR-100, SVHN, Food-101} \\
\hline
Optimizer & \multicolumn{1}{c}{AdamW \cite{loshchilov2017decoupled} }  \\
Base learning rate & \multicolumn{1}{c}{0.01} \\
Weight decay & \multicolumn{1}{c}{0.01} \\
Batch size & \multicolumn{1}{c}{128}  \\
Training crop size & \multicolumn{1}{c}{224} \\
Learning rate schedule & \multicolumn{1}{c}{Cosine decay~\cite{loshchilov2016sgdr}} \\
GPU numbers     & 1  \\
Warmup epochs & 20   \\
Training epochs & 100  \\
Augmentation & RandomResizedCrop  \\
\bottomrule
\end{tabular}

\end{table}

\noindent \textbf{Experimental settings on video datasets.}

We use two video datasets, Kinetics-400 (K400) \cite{carreira2017k400} and Something-Something V2 (SSv2) \cite{goyal2017ssv2}, to evaluate performance as the token count scales up. The experimental settings are shown in Table~\ref{video_experimental_table}. The number of input frames is set to 8. During testing, we use multi-view, a common practice in video action recognition. Experiments on others PEFT methods also follow these experimental settings.

\begin{table}[h]
    \caption{Experimental settings for complete video datasets. We follow most of settings in \cite{pan2022st}. The number of input frames is set to 8 in all experiments.}
    \label{video_experimental_table}
    \addtolength{\tabcolsep}{2pt}
    % \setstretch{0.80}
    
    \centering
    \scriptsize
    \begin{tabular}{lccc}
        \toprule
        Configuration & K400  & SSV2 \\ 

        \midrule
        Optimizer & \multicolumn{2}{c}{AdamW \cite{loshchilov2017decoupled}} \\

        Base learning rate & \multicolumn{2}{c}{1e-3} \\
        Weight decay & \multicolumn{2}{c}{0.01} \\
        Batch size & \multicolumn{2}{c}{128} \\
        Training epochs & 12  & 50 \\
        % training resize 
        lr
        % Learning rate & \multicolumn{2}{c}{$lr = base\_learning\_rate\times batch\_size / 256$} \\
        
        Training resize & \multicolumn{1}{c}{\begin{tabular}{cc}
        ShortSideJitter 
        \end{tabular}}  & \multicolumn{1}{c}{RandomResizedCrop} \\
        Training crop size & \multicolumn{2}{c}{224} \\
        
        Learning rate schedule & \multicolumn{2}{c}{Cosine decay~\cite{loshchilov2016sgdr}}     \\

        \midrule
        Num. testing views & \multicolumn{1}{c}{1 spatial $\times$ 3 temporal} & \multicolumn{1}{c}{3 spatial $\times$ 1 temporal} \\ 
        \bottomrule
    \end{tabular}

\end{table}

\section{Additional Experiments} \label{sup:additional exp}

In this section, we present additional ablation studies followed by a comprehensive comparison with mainstream PEFT methods on CIFAR-100 to evaluate the performance and efficiency of Sparse-Tuning for ViT adaptation.

\subsection{Visualizations of Different Irrelevant Token Processing Strategies.} We visualize the process of TC using different irrelevant token processing strategies, i.e., Drop and Merge (ours). As shown in Figure \ref{fig:sparsification_comparision}, directly dropping the semantic-irrelevant tokens can result in significant information loss. In contrast, merging these tokens mitigates this issue, thereby leading to improved performance. Consequently, in our actual implementation, we choose to merge the irrelevant tokens into a single representative token to compensate for potential information loss.

\begin{figure*}[t]
    \centering
    \includegraphics[width=\textwidth]{ICCV2025-Author-Kit-Feb/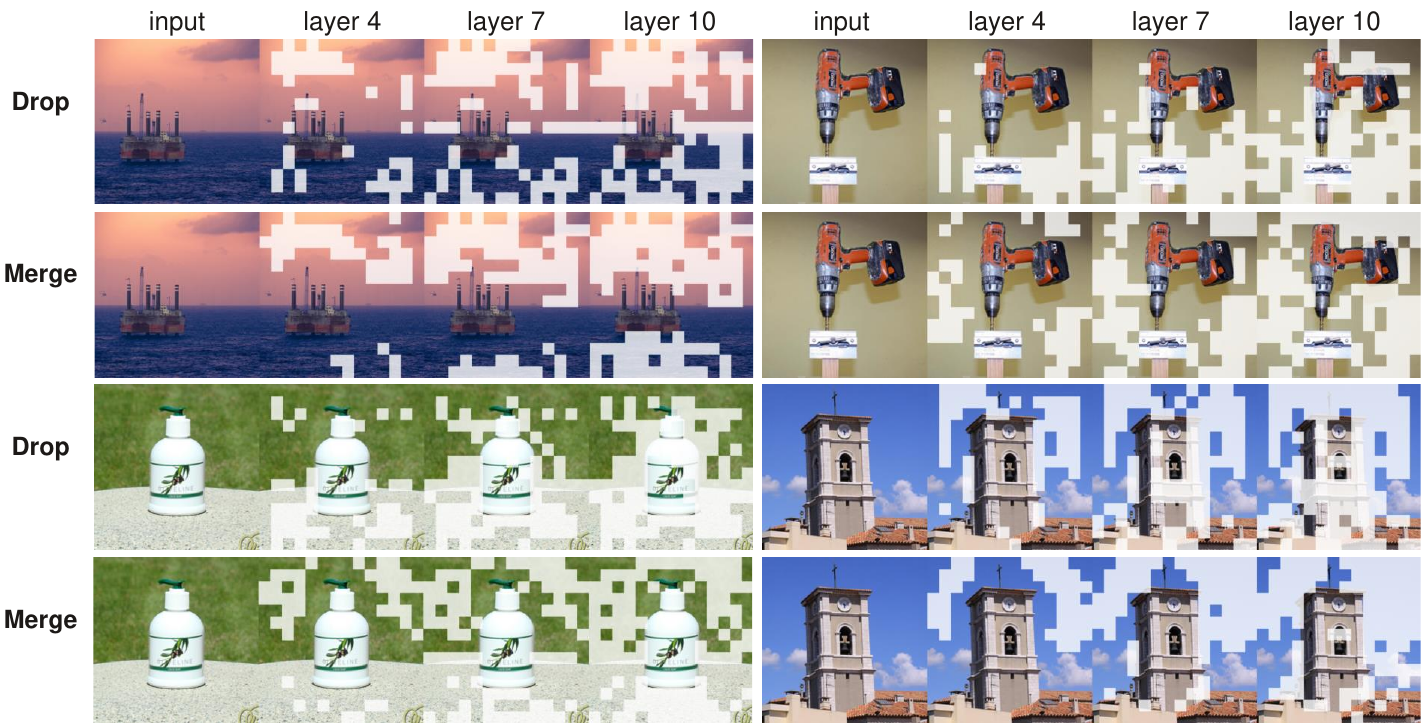}
    \vspace{-6mm}
    \caption{Visualizations of Different Irrelevant Token Processing Strategies. "Drop" refers to directly removing all irrelevant tokens, while "Merge" indicates merging the irrelevant tokens into a single representative token.}
\vspace{-3mm}
\label{fig:sparsification_comparision}
\end{figure*}

\subsection{Different Starting Layers of TC.} We explore different starting layers of TC to explore the optimal performance. From Table \ref{Table:sparsification boundary} (a,b), applying TC too early in shallow layers reduces accuracy, as ViT struggles to identify important tokens at these early stages due to unreliable attention maps. Similarly, from Table \ref{Table:sparsification boundary} (b,c), starting Token Sparsification too late in deeper layers also hurts accuracy, likely due to the loss of key token interactions. Therefore, we select to conduct TC in the 4-th encoder layers.

\input{ICCV2025-Author-Kit-Feb/Tables/boundary}

\subsection{Different Interval of Layers for TC.} We further explore the impact of different intervals between encoder layers when implementing TC, starting from the 4th encoder layer. From Table \ref{Table:sparsification interval}, we observe that shorter intervals (e.g., interval = 2) may lead to more frequent losses of visual information, thereby impairing performance. Conversely, longer intervals (e.g., interval = 4) may allow irrelevant tokens to persist for too long, leading to an accumulation of noise and less effective token reduction, which ultimately compromises feature representation and reduces accuracy. Based on these observations, we select an interval of 3 encoder layers in practical applications, achieving a balance between minimizing information loss and reducing irrelevant token retention.

\input{ICCV2025-Author-Kit-Feb/Tables/interval}

\subsection{Different Bottleneck Dimensions of DA.} We explore the impact of the bottleneck dimension $d$ of Dense Adapter in Sparse-Tuning to achieve the best trade-off between performance, updated parameters, and computational cost. As reported in Table \ref{Table:neck}, a higher bottleneck dimension $d$ introduces more parameters and higher GFLOPs. However, with a smaller $d$, the down-projection may lose significant information about the original features, leading to performance degradation. We observe that performance peaks at a bottleneck dimension of 32 and declines thereafter. Therefore, considering the trade-off between trainable parameters, GFLOPs, and performance, we set $d=32$.

\begin{table}[t]  
    \caption{Comparison of features from different layers in DA.}
    \label{tab:N-3}
    \centering
    \setlength{\tabcolsep}{5pt}
    \scalebox{1}{
    \begin{tabular}{lcccc}
        \toprule
        \# & Layer & GFLOPs & CIFAR-100 & Food-101 \\
        \midrule
        (a) & [N-1,N-2,N] & 11.66 & 90.39 & 89.22 \\
        \midrule
        (b) & [N-1,N-3,N] & 11.70 & \textbf{92.31} & \textbf{90.72} \\
        \bottomrule
    \end{tabular}}

\end{table}

\input{ICCV2025-Author-Kit-Feb/Tables/neck}

\input{ICCV2025-Author-Kit-Feb/Tables/CIFAR_100}

\subsection{Performance and Efficiency on CIFAR-100.} In Table \ref{tab:CIFAR-100}, we present the numbers of updated parameters during fine-tuning, GPU memory usage during both fine-tuning and inference, time for fine-tuning and inference, GFLOPs, and accuracy of our Sparse-Tuning method compared to other mainstream PEFT methods on the CIFAR-100 dataset \cite{krizhevsky2009cifar-100}. Evidently, our Sparse-Tuning achieves state-of-the-art performance while significantly enhancing efficiency during both the fine-tuning and inference stages.

\section{Pseudocode of Sparse-Tuning.} 

We present the PyTorch-like pseudocode of Sparse-Tuning in Algorithm \ref{alg:code} to help to better understand the whole process.

\input{ICCV2025-Author-Kit-Feb/Tables/code}

\section{More Visualizations of TC}
\label{sup:visualizations}

We present more visualization results of TC in Figure \ref{fig:token_sparsification_sup}. The results demonstrate that given various images, the TC in our Sparse-Tuning can effectively maintain the tokens from semantic-relevant foreground regions.

\begin{figure*}[h]
    \centering
    \includegraphics[width=\textwidth]{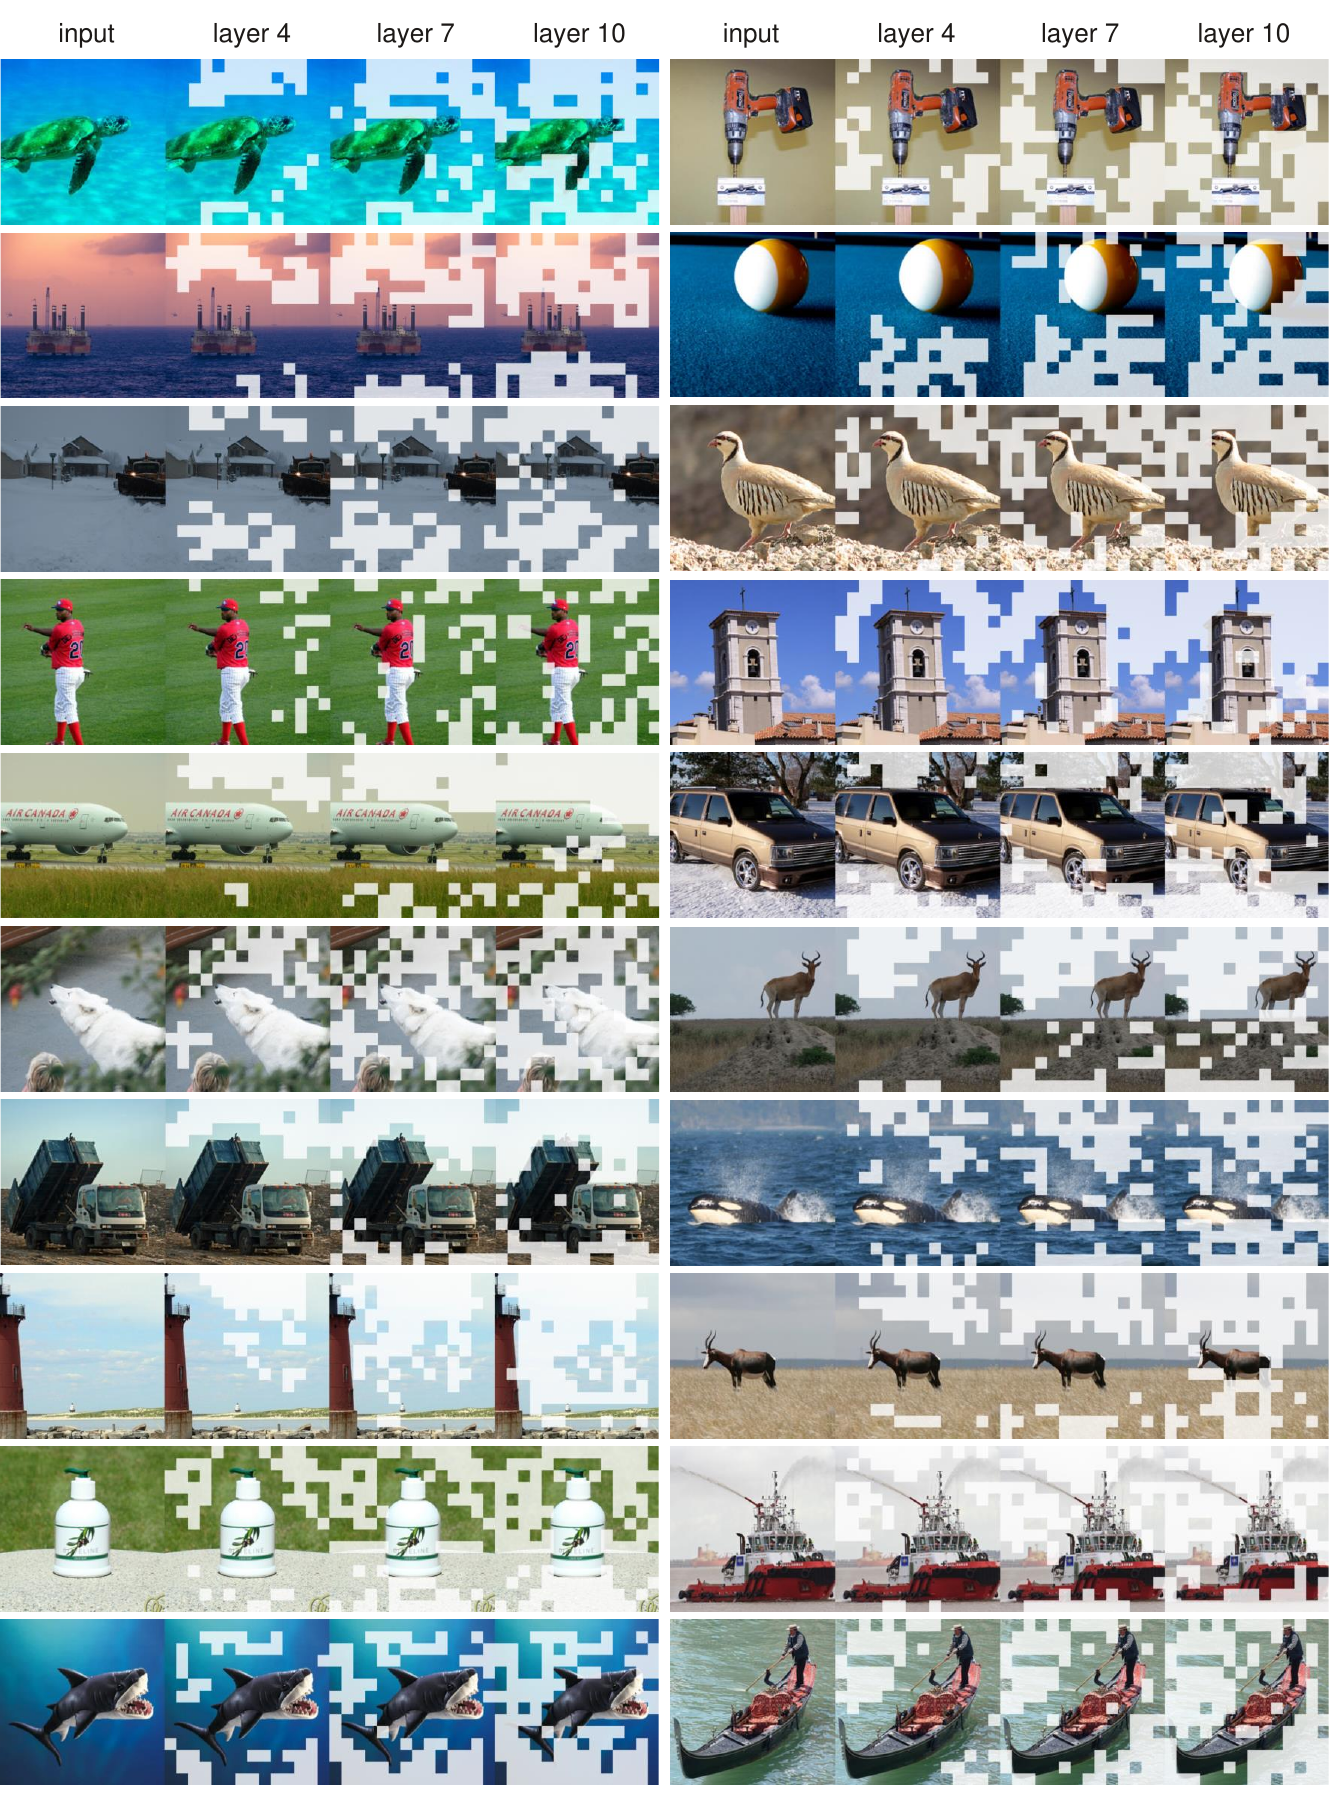}
    %\caption{\textbf{More visualizations of Token Sparsification by Dense-Tuning.}} 
    \caption{More visualizations of TC by Sparse-Tuning.} 
\vspace{-3mm}
\label{fig:token_sparsification_sup}
\end{figure*}

% \begin{table}[t]
%     \centering
%     \resizebox{0.48\linewidth}{!}{%
%     \begin{tabular}{cccc}
%         \toprule
%         \# & GFLOPs & CIFAR-100 & Food-101 \\
%         \midrule
%         [N-1,N-2,N] & 11.66 & 90.39 & 89.22 \\
%         \midrule
%         [N-1,N-3,N] & 11.70 & \textbf{92.31} & \textbf{90.72} \\
%         \bottomrule
%     \end{tabular}}
%     \caption{Comparison of features from different layers in DA.}
%     \label{tab:N-3}
% \end{table}
